# Supplementary material for: Strong Aharonov-Bohm quantum interference in simply-connected LaAlO$_3$/SrTiO$_3$ structures
Source: arXiv:1909.11259 source file (2019-10-17)
Supplement: Supplementary file 1 [file supplement.tex]

\documentclass[%
 reprint,
superscriptaddress,
%groupedaddress,
%unsortedaddress,
%runinaddress,
%frontmatterverbose, 
%preprint,
%showpacs,preprintnumbers,
%nofootinbib,
%nobibnotes,
%bibnotes,
 amsmath,amssymb,
 aps,
%pra,
prl,
%rmp,
%prstab,
%prstper,
floatfix,
]{revtex4-1}

\usepackage{graphicx}% Include figure files
\usepackage{dcolumn}% Align table columns on decimal point
\usepackage{bm}% bold math
\usepackage{xfrac}
\usepackage{txfonts}
\usepackage{siunitx}
\usepackage{upgreek}
%\usepackage{hyperref}% add hypertext capabilities
%\usepackage[mathlines]{lineno}% Enable numbering of text and display math
%\linenumbers\relax % Commence numbering lines

%\usepackage[showframe,%Uncomment any one of the following lines to test 
%%scale=0.7, marginratio={1:1, 2:3}, ignoreall,% default settings
%%text={7in,10in},centering,
%%margin=1.5in,
%%total={6.5in,8.75in}, top=1.2in, left=0.9in, includefoot,
%%height=10in,a5paper,hmargin={3cm,0.8in},
%]{geometry}

\begin{document}
\title{Supplemental Materials: Strong Aharonov-Bohm quantum interference in simply-connected LaAlO$_3$/SrTiO$_3$ structures}% Force line breaks with \\

\author{Patrick Irvin}
\affiliation{Department of Physics and Astronomy, University of Pittsburgh, Pittsburgh, PA 15260, USA}
\author{Hyungwoo Lee}
\author{Jung-Woo Lee}
\affiliation{Department of Materials Science and Engineering, University of Wisconsin-Madison, Madison, Wisconsin 53706, USA}
\author{Megan Briggeman}
\author{Shicheng Liu}
\author{Anil Annadi}
\author{Guanglei Cheng}
\author{Michelle Tomczyk}
\author{Jinanan Li}
\author{Mengchen Huang}
\affiliation{Department of Physics and Astronomy, University of Pittsburgh, Pittsburgh, PA 15260, USA}
\author{Chang-Beom Eom}
\affiliation{Department of Materials Science and Engineering, University of Wisconsin-Madison, Madison, Wisconsin 53706, USA}
\author{Jeremy Levy}
% \email{jlevy@pitt.edu}
\affiliation{Department of Physics and Astronomy, University of Pittsburgh, Pittsburgh, PA 15260, USA}

\date{\today}

\maketitle

\onecolumngrid
\renewcommand{\figurename}{FIG. S\!\!}

\begin{figure}[ht]
    \centering
    \includegraphics{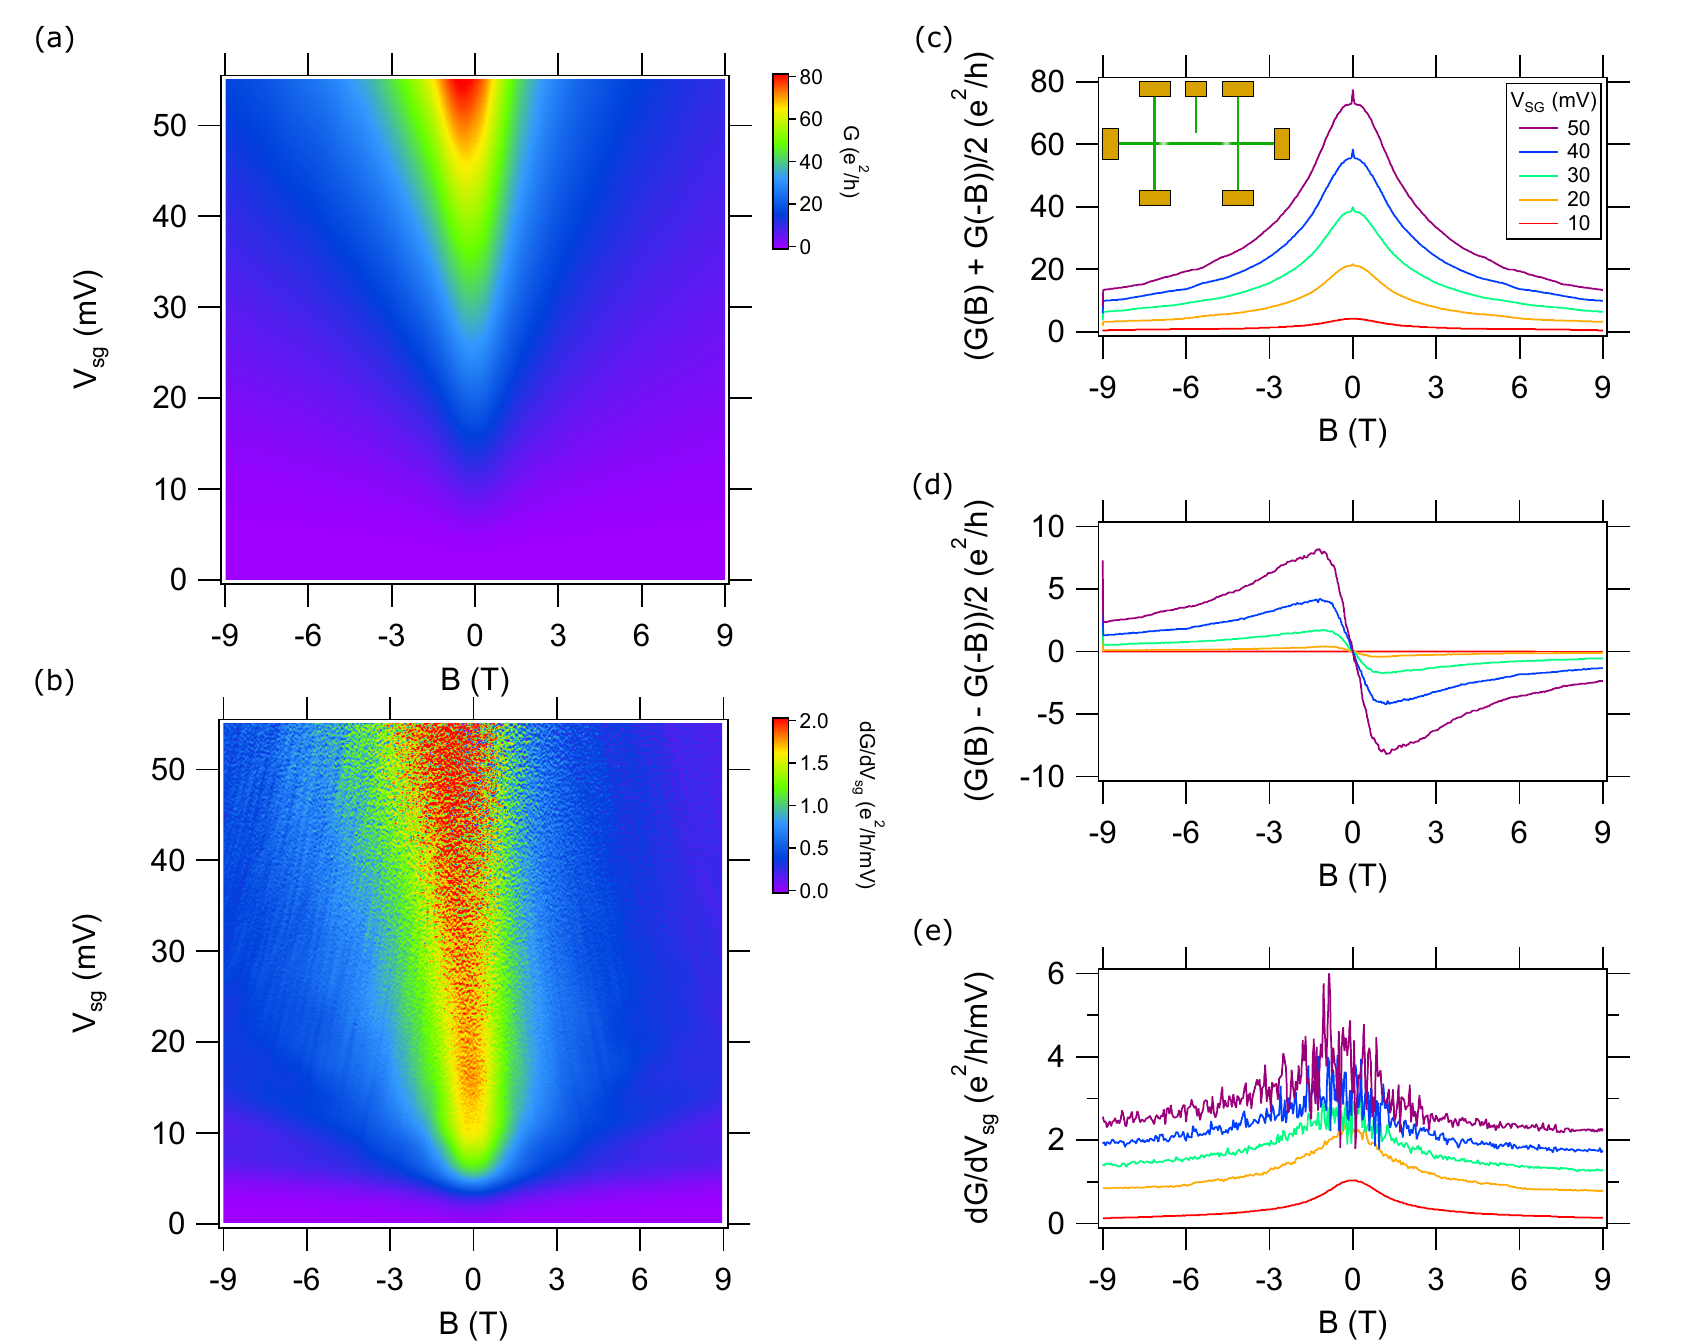}
    \caption{1D Electron waveguide at elevated temperature. (a) Conductance $G$ vs magnetic field $B$ and side gate $V_{sg}$. (b) Transconductance $dG/dV_{sg}$ showing interference effects. (c) Symmetric and (d) antisymmetric components of conductance for various values of $V_{sg}$. (e) Transconductance of various values of $V_{sg}$. $T = 600 \,\textnormal{mK}$.}
    \label{fig:figS1}
\end{figure}

\begin{figure}[ht]
    \centering
    \includegraphics{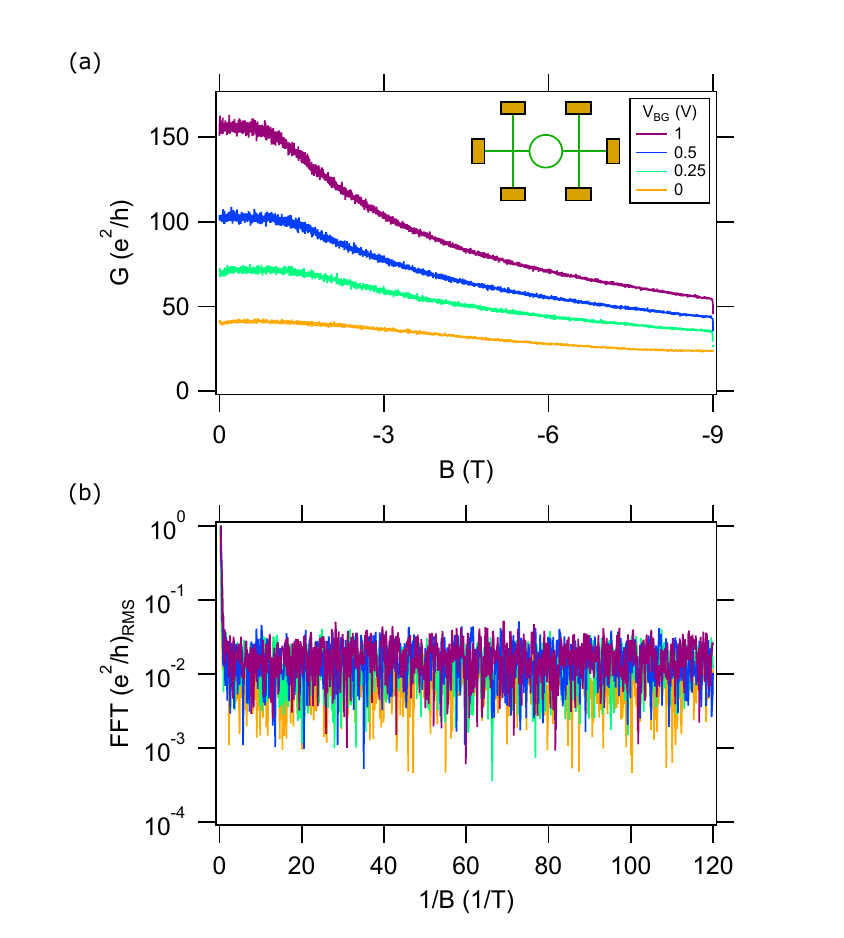}
    \caption{1D Ring. (a) Conductance versus magnetic field at several values of the back gate $V_{BG}$. (b) Corresponding power spectra. $A = \pi w_R^2 = 0.25 \,\upmu\textnormal{m}^2$, which has an expected oscillation period of 47 \si{\per\tesla}.}
    \label{fig:figS2}
\end{figure}

\end{document}
